# Supplementary material for: Analysis of the calculated X-X ro-vibrational transition intensities in molecular hydrogen
Source: arXiv:2308.10085 ancillary file (2023-08-19)

Supplementary material to paper by V.G. Ushakov, S.A. Balashev, and E.S. Medvedev "Analysis of the calculated X-X ro-vibrational transition intensities in molecular hydrogen".

Data from **Abgrall93L** and **Abgrall93W**.

Lyman series:

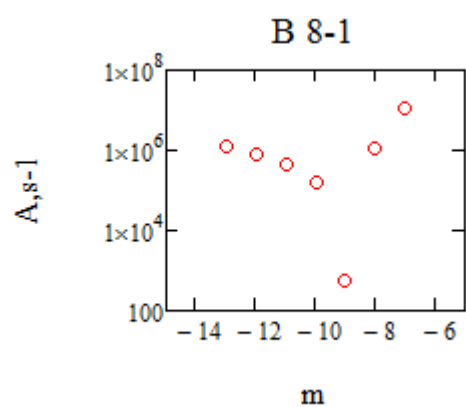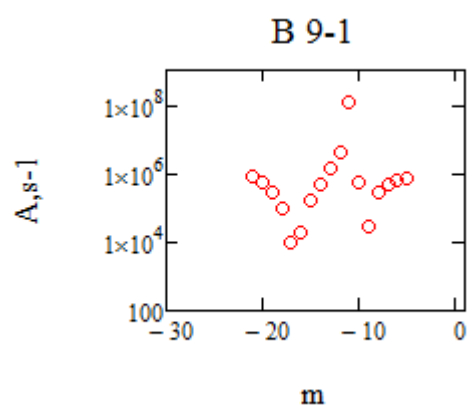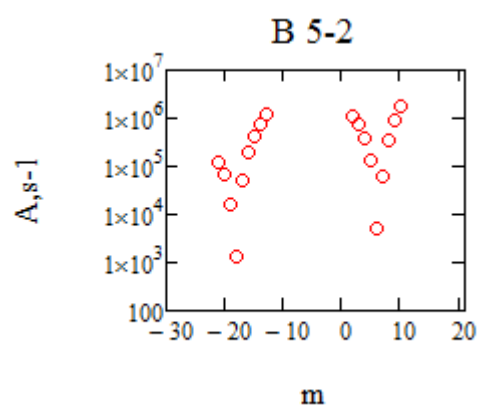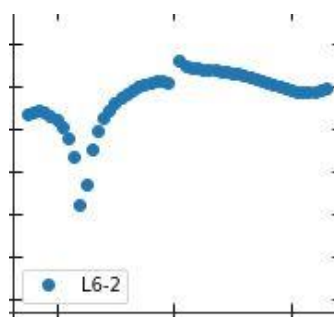

(not found in Table 1 of **Abgrall93L**).

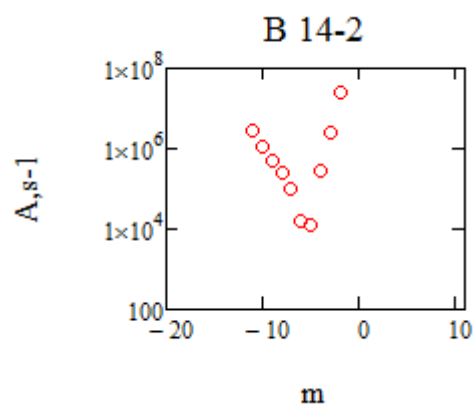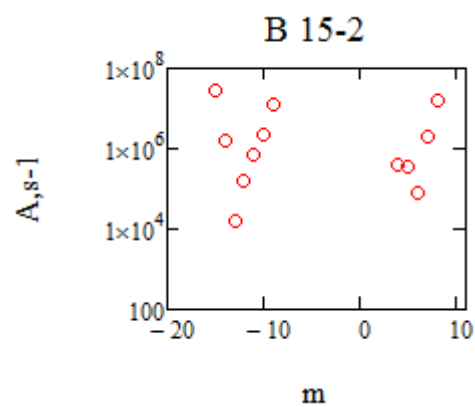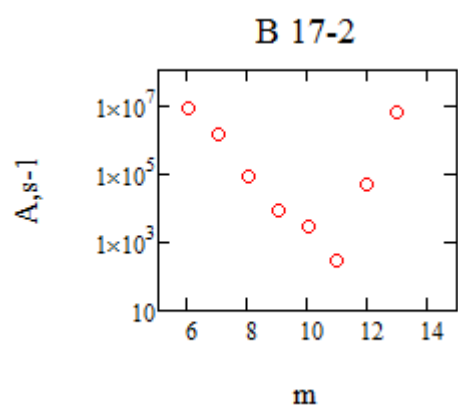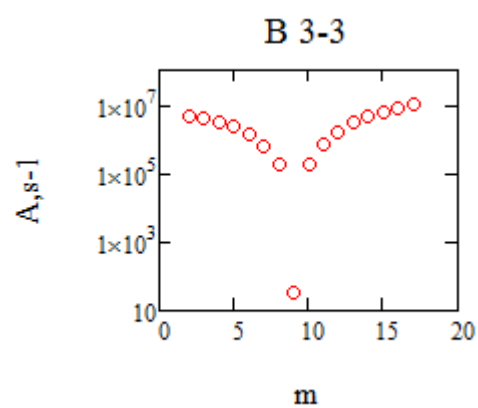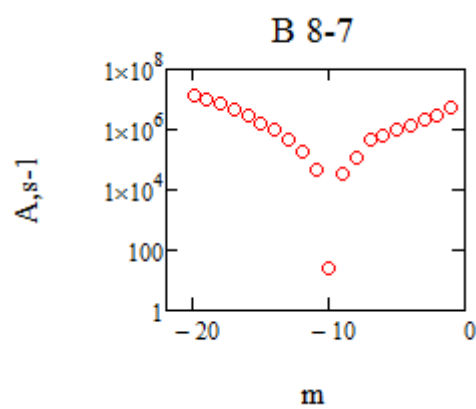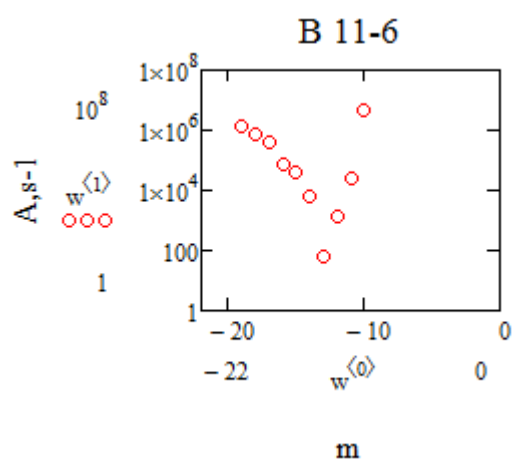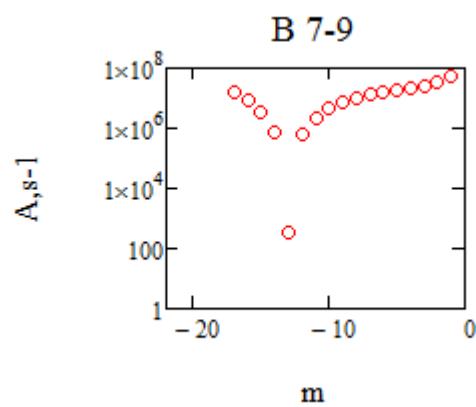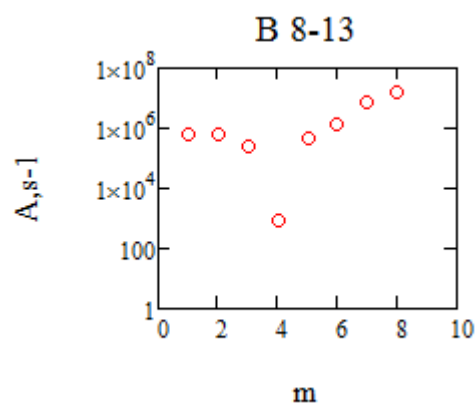

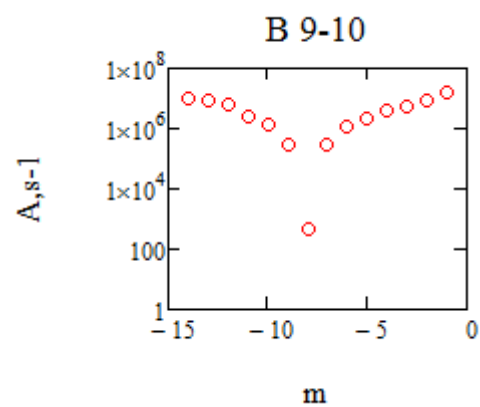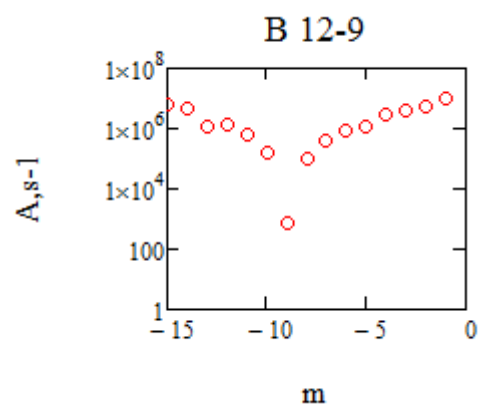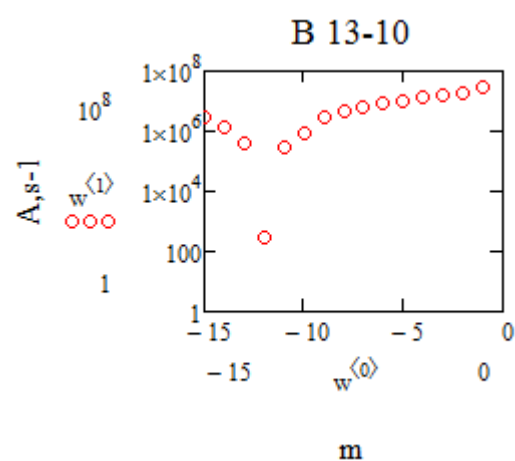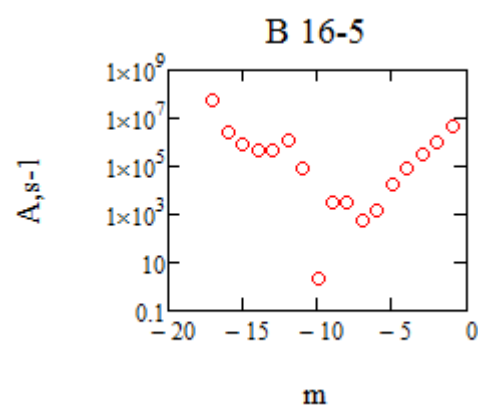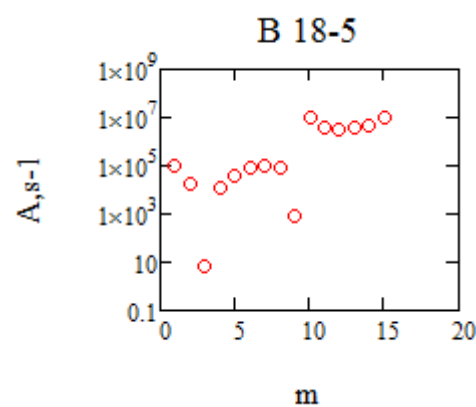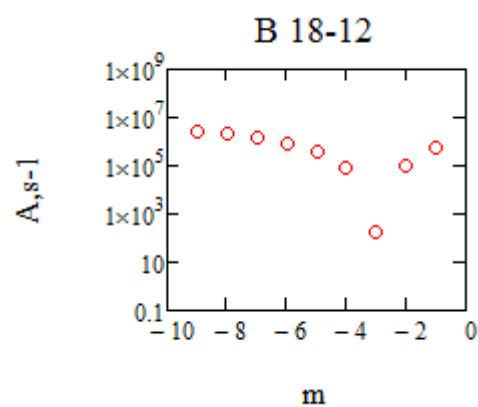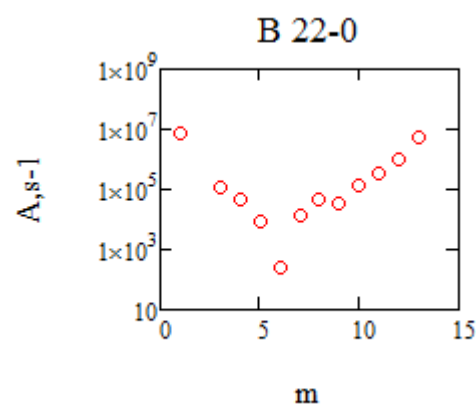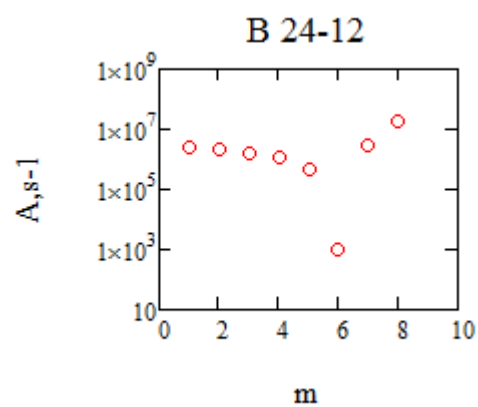

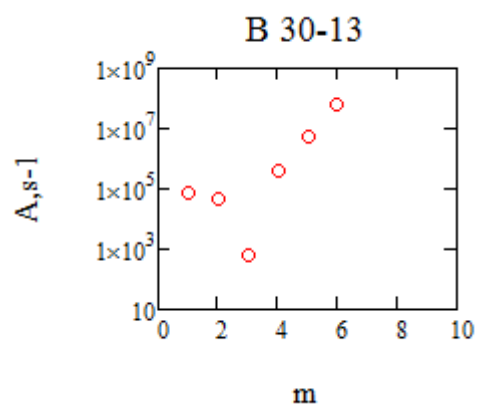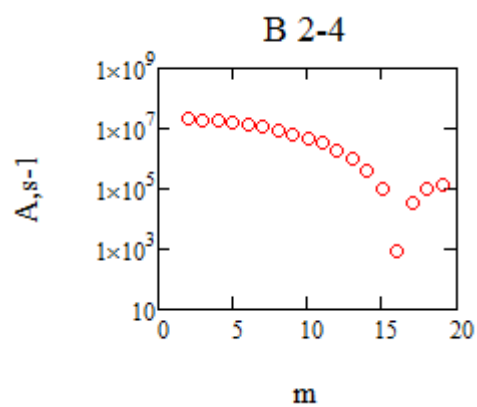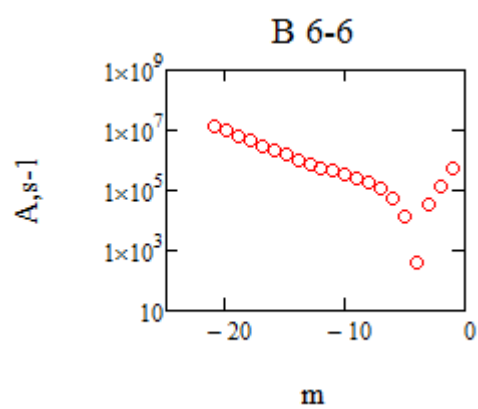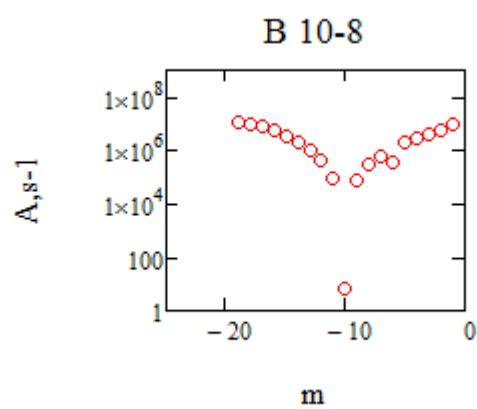

Werner series:

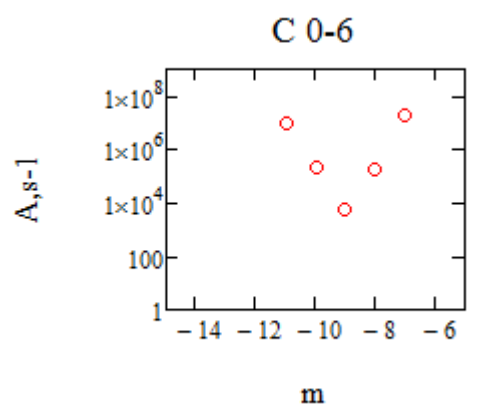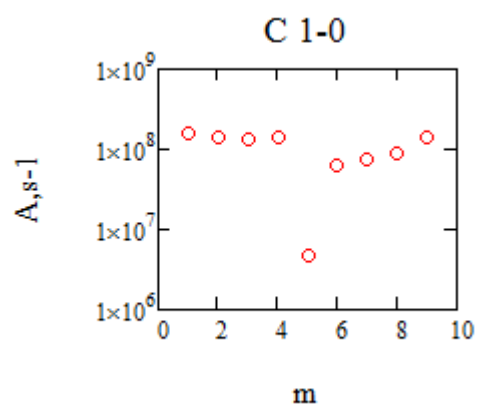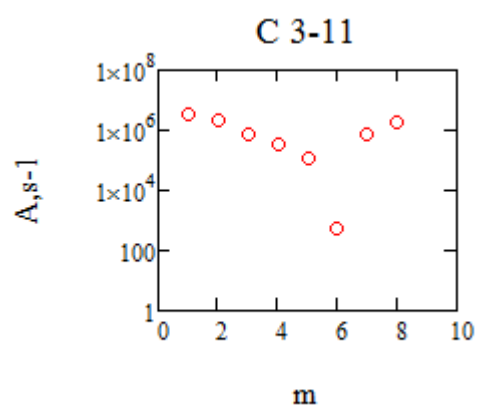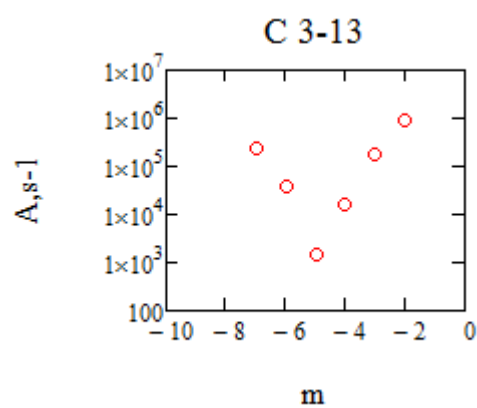

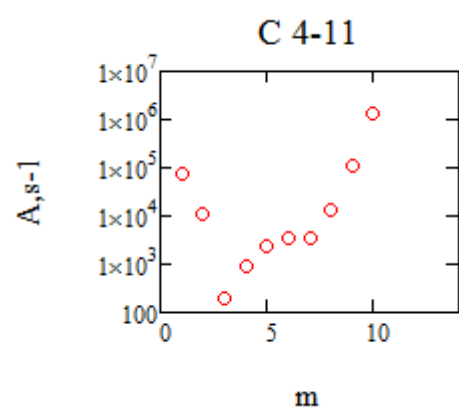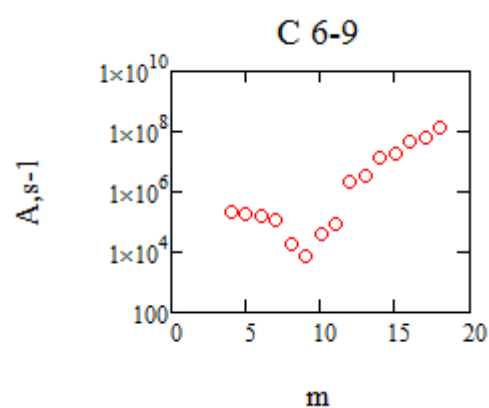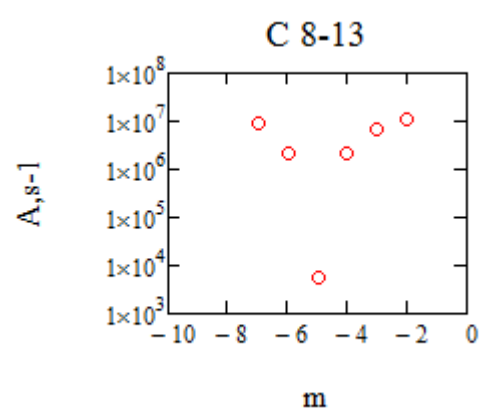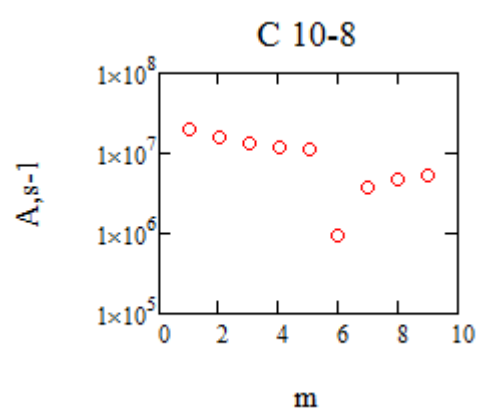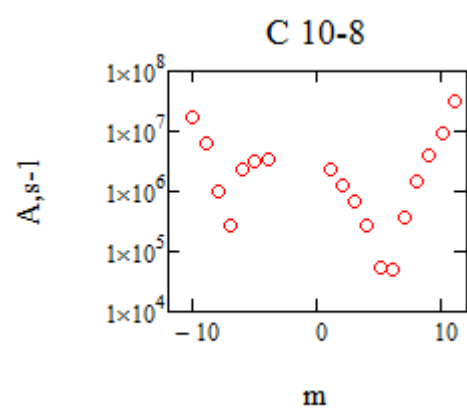

Supplement: Supplementary file 2 [file Anomalies_in_Lyman_and_Werner_series.pdf]
